# Supplementary material for: FedSecurity: Benchmarking Attacks and Defenses in Federated Learning and Federated LLMs
Source: arXiv:2306.04959 source file (2024-06-21)
Supplement: Supplementary file 1 [file appendix_ethics_statement.tex]

\section{Ethics Statement}\label{ethics}
FedSecurity %, as well as FedML and FedLLM, 
is under the Apache 2.0 license, ensuring open access and customization. %The code of conduct of the library is available at~\citep{fedml_code_of_conduct}. 
All datasets used for evaluations are publicly available, such as CIFAR10~\citep{cifar}, FEMNIST~\citep{caldas2018leaf}, Shakespeare~\citep{shakespeare}, and so on. All models for evaluations are publicly available as well.

\subsection{Code of Ethics}

% \textbf{Data and Model Ownership.}
% Any data uploaded by the users remains their property. Neither FedSecurity nor FedML does not claim ownership of any user data. If users employ the FedML platform (https://open.fedml.ai/) for model training, the resulting models and data remain the users' intellectual property.

\textbf{Data Handling and Protection.}
We are aware of the risks associated with data processing in FL settings. Users can use the open-sourced FedSecurity library %(FedML, FedLLM, and FedSecurity) 
to simulate attacks and defenses on any machine without uploading their raw data and model. 
If users use our MLOps platform for simulation, only the model weights are uploaded. The uploaded model weights are encrypted (\textit{i}.\textit{e}., only users with proper ownership can decrypt them) and can be deleted upon request. That is, %any FedML product, including the FedSecurity benchmark we propose in this work, 
we have no access to raw user data and we do not claim any data and model ownership.

\noindent\textbf{Benchmark Model Documentation and Transparency.}
% While we strive to protect the intellectual intricacies of our benchmark, we commit to:
We are committed to: \textit{i}) providing comprehensive documentation on the functionalities of the benchmark; \textit{ii}) making a detailed datasheet available for the benchmark model, outlining its specifications, capabilities, and intended use cases; and \textit{iii}) offering transparent and well-documented APIs for users.

\subsection{Limitations and Further Improvement}
While FedSecurity offers a foundation for ML security research, we recognize its limitations and potential for further enhancement. Our plans for improvement are as follows:
\textit{i}) conducting more experiments on federated LLMs to provide a comprehensive understanding of vulnerabilities of LLMs within the FL context; and \textit{ii}) designing and implementing advanced defense mechanisms against potential adversaries in asynchronous FL scenarios.

\subsection{Potential Negative Social Impacts}
Even though we put our best efforts in mitigating negative social impacts, the proposed FedSecurity benchmark might still be subject to some indistinct negative social impact, including:

\begin{itemize}
    \item \textbf{Potential misuse}: While our module simulates attacks and defenses in FL to help the communities to better understand and compare the attacks in FL, it is not immune to malicious use. The platform could potentially be used to exploit vulnerabilities or develop advanced attack techniques in FL systems.
    \item \textbf{Data security}: FL is susceptible to various threats such as data poisoning. We acknowledge these inherent risks and are actively working on introducing defenses mechanisms to mitigate such attacks.
    \item \textbf{Privacy Concerns}: Although FL aims to train models without sharing raw data, there remains a risk of indirect data leakage, for example, attackers might utilize the models to infer whether specific data points are in the training datasets, where users should be cautious and informed.
    
\end{itemize}
