# Supplementary material for: FedSecurity: Benchmarking Attacks and Defenses in Federated Learning and Federated LLMs
Source: arXiv:2306.04959 source file (2024-06-21)
Supplement: Supplementary file 2 [file appendix.tex]

\newpage
\appendix
\section*{Appendix}

% \section{Example Configuration Files for Attacks and Defenses}\label{exampleconfig}

% We provide example configuration files for Byzantine attack~\citep{chen2017distributed,fang2020local} in Figure~\ref{fig: attack_example} and for $m$-Krum defense~\citep{krum} in Figure~\ref{fig: defense_example}.

%  \begin{figure}[h]
%      \centering
%      \includegraphics[width=4cm]{figures/attack_examples.pdf}
%      % \vspace{-4mm}
%      \caption{Configuration for Byzantine attack~\citep{chen2017distributed,fang2020local}.}
%     \label{fig: attack_example}
%  \end{figure}

%  \begin{figure}[h]
%      \centering
%      \includegraphics[width=4cm]{figures/defense_examples.pdf}
%      % \vspace{-4mm}
%      \caption{Configuration for $m$-Krum~\citep{krum} defense.}
%     \label{fig: defense_example}
%  \end{figure}

%Results in Figure~\ref{fig:bert_exp} shows that $m$-Krum effectively mitigates the adversarial effect, bringing it closer to the level in the attack-free case, indicating the effectiveness of the $m$-Krum defense.

% \begin{figure}
%     \includegraphics[width=\textwidth]{figures/real_world_simulation.png}
%     \caption{Evaluations on Bert.}
%         \label{fig:bert_exp}
% \end{figure}

% \input{model_cards}

% \input{appendix_ethics_statement}
